# Supplementary material for: Magneto-optical response of the Weyl semimetal NbAs: Experimental results and hyperbolic-band computations
Source: arXiv:2312.03094 source file (2023-12-05)
Supplement: Supplementary file 1 [file sm.pdf]

# Magneto-optical response of the Weyl semimetal NbAs: Experimental results and hyperbolic-band computations SUPPLEMENTAL MATERIAL

S. Polatkan,<sup>1</sup> E. Uykur,<sup>1,2</sup> J. Wyzula,<sup>3</sup> M. Orlita,<sup>3,4</sup> C. Shekhar,<sup>5</sup> C. Felser,<sup>5</sup> M. Dressel,<sup>1</sup> and A. V. Pronin<sup>1</sup>

<sup>1</sup>*Physikalisches Institut, Universität Stuttgart, 70569 Stuttgart, Germany*

<sup>2</sup>*Institut für Ionenstrahlphysik und Materialforschung, HZDR, 01328 Dresden, Germany*

<sup>3</sup>*LNCMI, CNRS-UGA-UPS-INSA-EMFL, 38042 Grenoble, France*

<sup>4</sup>*Faculty of Mathematics and Physics, Charles University, 121 16 Prague, Czech Republic*

<sup>5</sup>*Max-Planck-Institut für Chemische Physik fester Stoffe, 01187 Dresden, Germany*

## Sec. I. Comparison with published results

Fig. S1 demonstrates the results of our measurements, dotted lines, together with the experimental results of Ref. [1], squares.

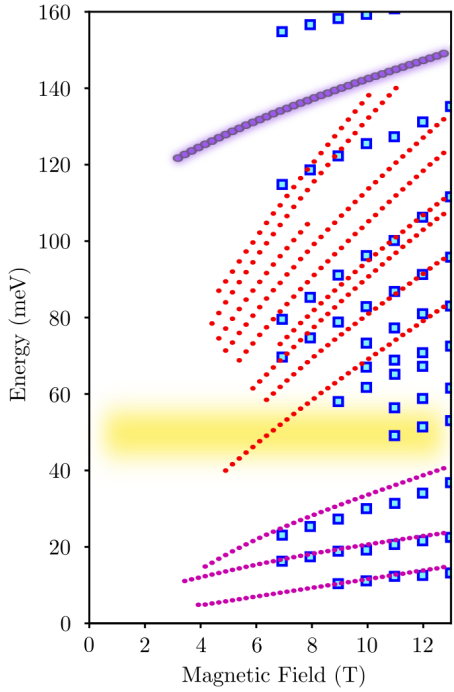

FIG. S1—Landau-level transitions observed in the magneto-optical  $R_B/R_0$  spectra of NbAs in this work (dotted lines) and in Ref. [1] (squares). The noise level around 50 meV is rather high in our measurements – this area is shaded yellow.

## Sec. II. Effect of different $v_z$ on the Landau-level spectrum

In Fig. S2, we show our calculations of the inter-Landau-level transitions for the model Hamiltonian discussed in the main text with two different velocities along the  $q_z$  momentum direction,  $10^4$  and  $10^5$  m/s. All other model parameters were kept identical. The calculations were made using the Kubo formula, see next Section. The difference in the out-of-plane velocities leads to a difference in the joint density of states:  $\rho(E) = 2/(\hbar v_z)$  (a linear dispersion along  $q_z$  is assumed).

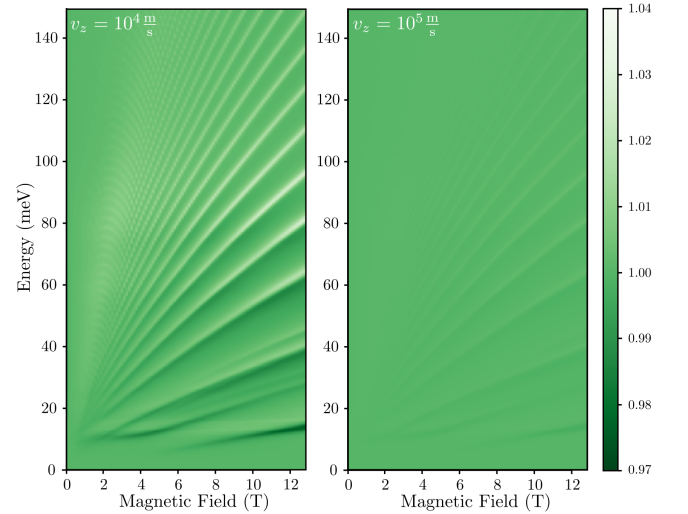

FIG. S2—Relative reflectivity calculated for different Fermi velocities  $v_z$  as indicated. A larger  $v_z$  implies a lower density of states, reducing the strength of the Landau-level features.

## Sec. III. Optical conductivity and reflectivity calculations

The interband complex optical conductivity was calculated using a Kubo formula:

$$\sigma^\pm(\omega, B) = \frac{iG_0}{l_B^2 \omega} \sum_{n,m,q_z} \frac{(f_m - f_n) |\langle m | \hat{v}_\pm | n \rangle|^2}{E_n - E_m - \hbar\omega + i\Gamma}, \quad (1)$$

where  $\sigma^\pm$  is the optical conductivity for circular polarizations of light,  $G_0 = e^2/h$  is the conductance quantum,  $l_B = \sqrt{\hbar/|eB|}$  is the magnetic length,  $f_{m,n}$  are the Fermi-Dirac functions for bands  $m$  and  $n$ , and  $\hat{v}_\pm = (\hat{v}_x \pm i\hat{v}_y)/\sqrt{2}$

are velocity operators, with  $\hbar\hat{v}_{x_i} = \partial\hat{H}/\partial q_{x_i}$ . We used  $T = 0$  K and the broadening parameter  $\Gamma = 1$  meV. Following Ref. [2], we considered states near  $q_z = 0$  and replaced the sum over  $q_z$  with the integrated joint density of states for a linear band,  $2\Gamma/(\hbar v_z)$ . For the model calculations presented in the main text,  $v_z = 10^4$  m/s was adopted from Refs. [3, 4]. The optical reflectivity was calculated from the complex conductivity via the standard optical formulas for normal incidence [5]:

$$R(\omega) = \frac{|\sqrt{\varepsilon(\omega)} - 1|^2}{|\sqrt{\varepsilon(\omega)} + 1|^2}, \quad \varepsilon(\omega) = 1 + \frac{i\sigma(\omega)}{\varepsilon_0\omega}. \quad (2)$$

To bring the calculated relative reflectivity response within range of our experimental data, i.e., near  $R_B/R_0 = 1$ , a finite amount of carriers had to be considered to conduct freely, not to be bound to the Landau levels. Therefore, we added the experimentally obtained zero-field complex conductivity of NbAs,  $\sigma_{\text{meas}}^{ZF}(\omega)$ , to the calculated optical conductivity of the Landau levels,  $\sigma_{\text{LL}}(\omega)$ . Thus, the total  $\sigma(\omega)$  in Eq. (2) was  $\sigma(\omega) = \alpha\sigma_{\text{meas}}^{ZF}(\omega) + (1 - \alpha)\sigma_{\text{LL}}(\omega)$ . We obtained reasonable values of  $R_B/R_0$  taking  $\alpha = 30$  to 40 % as free carriers and  $(1 - \alpha) = 60$  to 70 % as bound to Landau levels. For the calculations shown in this paper,  $\alpha$  was 35 %. Broadband optical conductivity of our NbAs sample was measured in advance and is shown in Fig. S3.

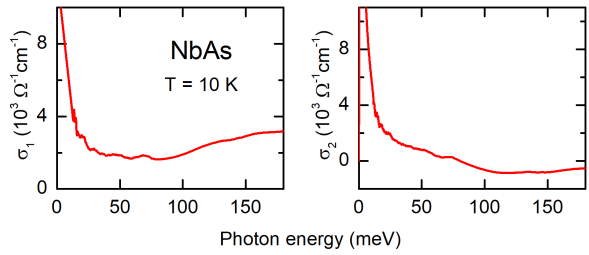

FIG. S3–Optical conductivity of the studied NbAs sample at 8 K. The lines below  $\sim 10$  meV are extrapolations according to the Drude model using the experimentally measured dc resistivity.

#### Sec. IV. Effect of different couplings on the Landau-level spectrum

Fig. S4 shows the inter-Landau-level spectrum of the model Hamiltonian for different coupling parameters. The spectrum of panel (a) corresponds to the model with presence of Weyl cones, discussed in the main text, with a negative  $c_4$ . Panel (b) shows the situation for Dirac cones with the SOC coupling parameters set to zero. From comparing panels (a) and (b), it is evident that the SOC only affects the low-energy portion of the spectrum, below 40 meV. In panel (c), the situation for a positive  $c_4$  is illustrated, which gaps out the cones. From panels (a) and (c) it becomes apparent that  $c_3$  splits the lowest transition line into two, in accordance with experimental observations. Evidently, since  $c_4$  is small, the difference between the low-energy transitions of the spectra (a) and (c) is insubstantial. Thus, both (a) and (c) reproduce the measured Landau levels well, underlining once more that the small Weyl cones do not contribute directly to the spectrum.

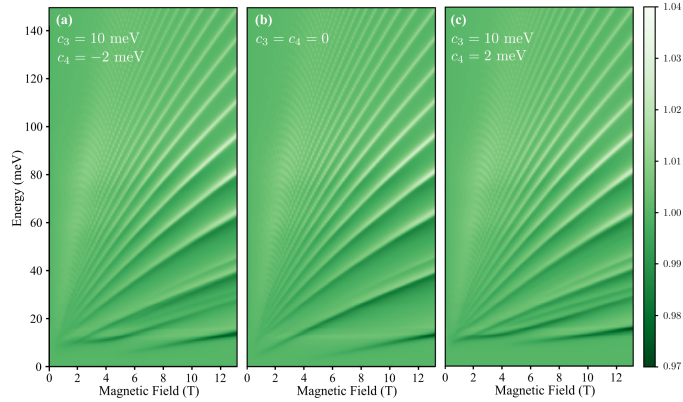

FIG. S4–Relative reflectivity calculated for different couplings. Panel (a): Same parameters as in the main text, the model bands structure hosts small Weyl cones. Panel (b): No Weyl nodes, only Dirac nodes. Panel (c): Slightly gapped band structure, no crossing bands.

### Sec. V. Uncertainty estimation for the model Hamiltonian parameters

The model parameters can be varied within a finite range of values, yielding qualitatively similar results. Here we provide estimates for the ranges, beyond which the calculated magneto-optical reflectivity does not fit reasonably well to the experimental data anymore. Naturally, some of the parameters should be tuned simultaneously to give a sensible estimate. For example, an estimate for the mass  $m$ , tuned together with the splitting parameter  $c_1$ , as to keep the overlap of the electron and hole bands constant, allows a larger range of values for  $m$  than if it was tuned while keeping  $c_1$  constant. In Table I, we list these, i.e, the largest uncertainties and indicate the sets of parameters that were simultaneously tuned. All units are in meV, except for the velocities.

| Parameters | Coupled Parameters | Uncertainties                                       |
|------------|--------------------|-----------------------------------------------------|
| $m$        | $c_1, v$           | $\Delta m = +30, -20$                               |
| $v_x$      | $m, c_1$           | $\Delta v_x = +7 \cdot 10^4; -5 \cdot 10^4$ m/s     |
| $v_y$      | $m, c_1$           | $\Delta v_y = +3.6 \cdot 10^4; -2.6 \cdot 10^4$ m/s |
| $c_1$      | $v, c_2$           | $\Delta c_1 = \pm 25$                               |
| $c_2$      | $v, c_1$           | $\Delta c_2 = \pm 25$                               |
| $c_3$      | $c_4$              | $\Delta c_3 = +10; -30$                             |
| $c_4$      | $c_3$              | $\Delta c_4 = +20; -15$                             |

TABLE SI–Uncertainties for the model parameters.

The constants  $c_3$  and  $c_4$  seem to allow a large amount of variation. However, it is important that they are tuned such that the intersect or the gap between the center electron and hole bands remains roughly of the same size as for the initial set of parameters. Otherwise, a gap (or an inverted gap) becomes immediately obvious in the spectrum and the experimental low-energy transitions cannot be fitted.

### Sec. VI. Landau quantization

The Peierls substitution in the Landau gauge reads  $(\hat{p}_x, \hat{p}_y) \rightarrow (\hat{p}_x, \hat{p}_y + eB\hat{x})$ . The ladder operators are defined as  $a^\dagger = \frac{l_B}{\sqrt{2}\hbar}(\hat{p}_x + i(\hat{p}_y + eB\hat{x}))$  and  $a = \frac{l_B}{\sqrt{2}\hbar}(\hat{p}_x - i(\hat{p}_y + eB\hat{x}))$  with the magnetic length  $l_B = \sqrt{\hbar/|eB|}$  and the commutation relation  $[\hat{a}^\dagger, \hat{a}] = \hat{a}^\dagger \hat{a} - \hat{a} \hat{a}^\dagger = 1$ . Thus, to obtain the quantized version of our model Hamiltonian (Eqs. (1) and (3) in the main text), the momenta should be replaced with:

$$\hat{p}_x \rightarrow \frac{\hbar}{\sqrt{2}l_B}(\hat{a} + \hat{a}^\dagger), \quad \hat{p}_y \rightarrow \frac{i\hbar}{\sqrt{2}l_B}(\hat{a} - \hat{a}^\dagger). \quad (3)$$

For example, if  $v_x = v_y = v$ , the Hamiltonian  $H_4$  becomes:

$$H_4 = \begin{pmatrix} m + c_1 & c_2 & 0 & v(\hat{p}_x - i\hat{p}_y) \\ c_2 & m - c_1 & v(\hat{p}_x + i\hat{p}_y) & 0 \\ 0 & v(\hat{p}_x - i\hat{p}_y) & -m - c_1 & -c_2 \\ v(\hat{p}_x + i\hat{p}_y) & 0 & -c_2 & -m + c_1 \end{pmatrix} \rightarrow \begin{pmatrix} m + c_1 & c_2 & 0 & \frac{\sqrt{2}\hbar v}{l_B}a \\ c_2 & m - c_1 & \frac{\sqrt{2}\hbar v}{l_B}a^\dagger & 0 \\ 0 & \frac{\sqrt{2}\hbar v}{l_B}a & -m - c_1 & -c_2 \\ \frac{\sqrt{2}\hbar v}{l_B}a^\dagger & 0 & -c_2 & -m + c_1 \end{pmatrix}. \quad (4)$$

### Sec. VII. Landau-level spectrum

In Fig. S5, the Landau-level spectrum for the model Hamiltonian with the parameters from the main text is shown. The Landau levels are labeled with the corresponding Landau-level indices  $n = 0, 1, 2, \dots$  and with superscripts “+” and “−” for the spin splitting. The transitions observed in  $R_B/R_0$  for  $|m| \rightarrow |n|$  are labeled only for  $|n| - |m| \geq 0$ . The transitions we observe are not always with  $|n - m| = 1$ . This is not unusual for Weyl semimetals and has been detected in NbP [6, 7].

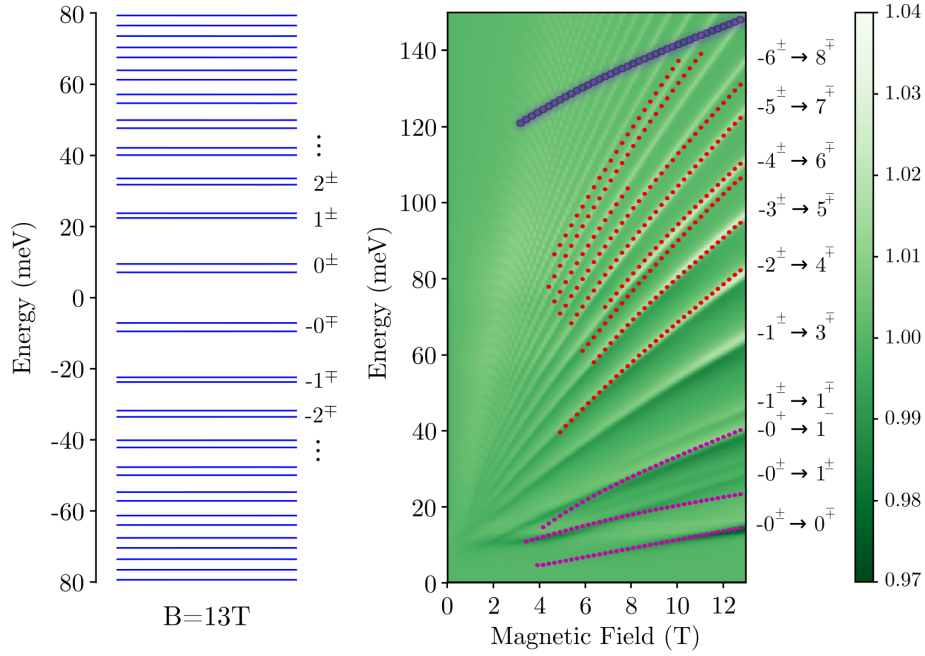

FIG. S5—The Landau-level spectrum (left) of the model Hamiltonian at  $B = 13$  T and the relative reflectivity  $R_B/R_0$  with labeled interband transitions (right).

- 
- [1] X. Yuan, Z. Yan, C. Song, M. Zhang, Z. Li, C. Zhang, Y. Liu, W. Wang, M. Zhao, Z. Lin, T. Xie, J. Ludwig, Y. Jiang, X. Zhang, C. Shang, Z. Ye, J. Wang, F. Chen, Z. Xia, D. Smirnov, X. Chen, Z. Wang, H. Yan, and F. Xiu, Chiral Landau levels in Weyl semimetal NbAs with multiple topological carriers, *Nat. Commun.* **9**, 1854 (2018).
  - [2] S. Polatkan, M. O. Goerbig, J. Wyzula, R. Kemmler, L. Z. Maulana, B. A. Piot, I. Crassee, A. Akrap, C. Shekhar, C. Felser, M. Dressel, A. V. Pronin, and M. Orlita, Magneto-optics of a Weyl semimetal beyond the conical band approximation: Case study of TaP, *Phys. Rev. Lett.* **124**, 176402 (2020).
  - [3] C.-C. Lee, S.-Y. Xu, S.-M. Huang, D. S. Sanchez, I. Belopolski, G. Chang, G. Bian, N. Alidoust, H. Zheng, M. Neupane, B. Wang, A. Bansil, M. Z. Hasan, and H. Lin, Fermi surface interconnectivity and topology in Weyl fermion semimetals TaAs, TaP, NbAs, and NbP, *Phys. Rev. B* **92**, 235104 (2015).
  - [4] D. Grassano, O. Pulci, A. M. Conte, and F. Bechstedt, Validity of Weyl fermion picture for transition metals monpnictides TaAs, TaP, NbAs, and NbP from *ab initio* studies, *Sci. Rep.* **8**, 3534 (2018).
  - [5] M. Dressel and G. Grüner, *Electrodynamics of Solids* (Cambridge University Press, 2002).
  - [6] Y. Jiang, Z. Dun, S. Moon, H. Zhou, M. Koshino, D. Smirnov, Z. Jiang, R. J. Cava, A. Vishwanath, and A. Yazdani, Landau quantization in coupled Weyl points: A case study of semimetal NbP, *Nano Lett.* **18**, 7726 (2018).
  - [7] M. Zhao, Z. Yan, X. Xie, Y. Yang, P. Leng, M. Ozerov, D. Yan, Y. Shi, J. Yang, F. Xiu, and S. Dong, Unconventional Landau level transitions in Weyl semimetal NbP, *Phys. Rev. Mater.* **6**, 054204 (2022).
